# Supplementary material for: FairVision: Equitable Deep Learning for Eye Disease Screening via Fair Identity Scaling
Source: arXiv:2310.02492 source file (2024-04-12)
Supplement: Supplementary file 1 [file appendix.tex]

\appendix
\section{Appendix}

\subsection{Computational Cost for Training}

Training an EfficientNet for 10 epochs in the AMD detection task requires 66 milliseconds per SLO fundus image and 833 milliseconds for an OCT B-scan. On the other hand, when training an EfficientNet with the proposed FIS for the same task, it takes 71 milliseconds per SLO fundus image and 901 milliseconds for an OCT B-scan. This indicates a slight increase in training time with the FIS method compared to the baseline EfficientNet, due to the additional fairness-related computations involved in FIS.

\subsection{Effects of Various Backbone Models}

% Figure \ref{fig:ablation_backbones} shows the comparison of performance across various backbone models for AMD detection using SLO fundus images and OCT B-scans w.r.t. the racial identity. As can be seen, EfficientNet achieves the best performance on the SLO fundus images. In contrast to 2D imaging modality SLO fundus image, OCT B-scans are a 3D imaging modality. Therefore, a CNN based on 3D convolutional modules would be a natural choice. By treating 3D OCT B-scans as 2D image with N ($\gg$ 3) channel, conventional deep learning models with 2D convolutional modules are able to apply to 3D OCT B-scans. However, according to Figure \ref{fig:ablation_backbones}, we can see that a simple 3D CNN outperforms the other models. This confirms the alignment between the 3D imaging modality and the 3D convolutional operation.

\textbf{Figure \ref{fig:ablation_backbones}} presents a performance comparison among various backbone models for AMD detection using both SLO fundus images and OCT B-scans in relation to racial identity. EfficientNet demonstrates superior performance in SLO fundus images, a 2D imaging modality. In contrast, since OCT B-scans represent a 3D imaging modality, one might consider using a CNN with 3D convolutional modules. As indicated in \textbf{Figure \ref{fig:ablation_backbones}}, a straightforward 3D CNN surpasses other models, underscoring the compatibility between the 3D imaging modality and 3D convolutional operations.

\begin{figure}[!h]
	\centering
	\subfloat[]{\includegraphics[width=0.4\textwidth]{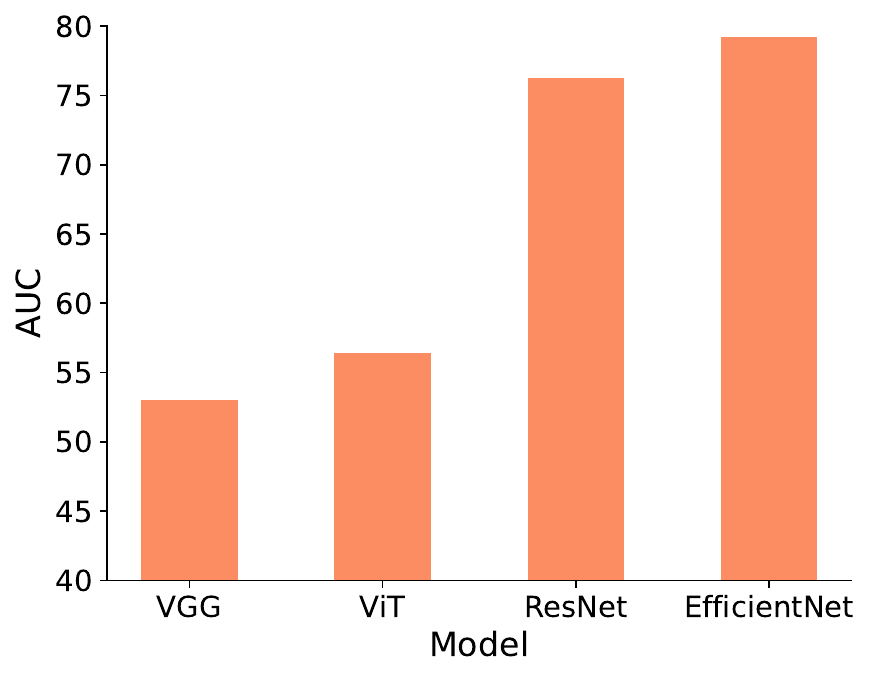}} \hspace{3ex}
	\subfloat[]{\includegraphics[width=0.4\textwidth]{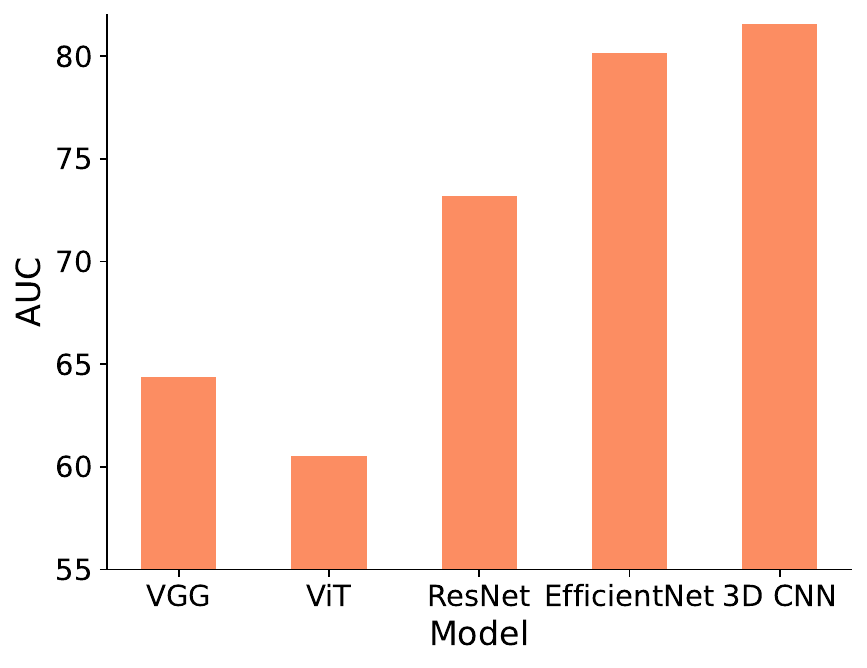} }  
	\caption{\label{fig:ablation_backbones}
    	Comparison of performance across different backbone models for AMD detection using SLO fundus images (a) and OCT B-scans (b) w.r.t. the racial identity.
    	}
     % [width=0.23\textwidth]
\end{figure}
